# Supplementary material for: Quantum Geometric Tensor for Mixed States Based on the Covariant Derivative
Source: arXiv:2506.00347 source file (2025-05-31)
Supplement: Supplementary file 1 [file supplementary_material_of_MSQGT__CPL_.pdf]

# Supplementary Material: Quantum Geometric Tensor for Mixed States based on the Covariant Derivative

Qianyi Wang, Ben Wang,[*] Jun Wang, and Lijian Zhang[†]
*National Laboratory of Solid State Microstructures,*
*Key Laboratory of Intelligent Optical Sensing and Manipulation,*
*College of Engineering and Applied Sciences and school of physics,*
*and Collaborative Innovation Center of Advanced Microstructures, Nanjing University, Nanjing 210093, China*
(Dated: May 30, 2025)

## DERIVATION OF THE EQUALITY BETWEEN THE IMAGINARY PART OF OUR MIXED-STATE QUANTUM GEOMETRIC TENSOR (MSQGT) AND THE MEAN GAUGE CURVATURE

Consider the mixed state

$$\rho = \sum_i p_i \, |\xi_i\rangle\langle\xi_i|, \tag{1}$$

for which we compute the gauge curvature. Suppose that a purification of $\rho$ is given by

$$|\psi\rangle = \sum_i \sqrt{p_i}\, |\xi_i\rangle \, |v_i\rangle, \tag{2}$$

where $\{|v_i\rangle\}$ denotes an orthonormal basis for the environmental Hilbert space. For the sake of notational convenience in the subsequent derivation, we introduce the following notations:

$$\alpha_{ik} \equiv \frac{2\sqrt{p_i p_k}}{p_i + p_k}, \qquad \beta_{ki,\mu} \equiv \langle \xi_k | \partial_\mu \xi_i \rangle, \qquad \gamma_{ki,\mu} \equiv \langle v_k | \partial_\nu v_i \rangle. \tag{3}$$

The covariant derivative can be expressed as

$$|D_\mu \psi\rangle = \sum_i \partial_\mu \sqrt{p_i} |\xi_i\rangle |v_i\rangle - \sum_{ik} \sqrt{p_k} \alpha_{ik} \beta_{ki,\mu} |\xi_k\rangle |v_i\rangle + \sum_i \sqrt{p_i} |\partial_\mu \xi_i\rangle |v_i\rangle. \tag{4}$$

$$\langle D_\nu \psi| = \sum_j \partial_\nu \sqrt{p_j} \langle \xi_j | \langle v_j| + \sum_{jl} \sqrt{p_l} \alpha_{jl} \beta_{jl,\nu} \langle \xi_l | \langle v_j| + \sum_j \sqrt{p_j} \langle \partial_\nu \xi_j | \langle v_j|. \tag{5}$$

The expression for our mixed-state quantum geometric tensor (MSQGT) can be expressed as

$$\begin{aligned}
Q_{\nu\mu} &= \langle D_\nu \psi | D_\mu \psi \rangle \\
&= \sum_i \partial_\nu \sqrt{p_i} \partial_\mu \sqrt{p_i} + \sum_i \sqrt{p_i} \partial_\mu \sqrt{p_i} \beta_{ii,\nu} - \sum_i \sqrt{p_i} \partial_\mu \sqrt{p_i} \beta_{ii,\nu} \\
&\quad - \sum_i \sqrt{p_i} \partial_\nu \sqrt{p_i} \beta_{ii,\mu} - \sum_{ik} p_k \alpha_{ik}^2 \beta_{ki,\mu} \beta_{ik,\nu} + \sum_{ik} \sqrt{p_k} \sqrt{p_i} \alpha_{ik} \beta_{ki,\mu} \beta_{ik,\nu} \\
&\quad + \sum_i \sqrt{p_i} \partial_\nu \sqrt{p_i} \beta_{ii,\mu} + \sum_{ik} \sqrt{p_i p_k} \alpha_{ik} \beta_{ik,\nu} \beta_{ki,\mu} + \sum_i p_i \langle \partial_\nu \xi_i | \partial_\mu \xi_i \rangle \\
&= \sum_i \partial_\nu \sqrt{p_i} \partial_\mu \sqrt{p_i} + \sum_i p_i \langle \partial_\nu \xi_i | \partial_\mu \xi_i \rangle + \sum_{ik} (-p_k \alpha_{ik}^2 + 2\sqrt{p_i p_k} \alpha_{ik}) \beta_{ik,\nu} \beta_{ki,\mu} \\
&= \sum_i \partial_\nu \sqrt{p_i} \partial_\mu \sqrt{p_i} + \sum_i p_i \langle \partial_\nu \xi_i | \partial_\mu \xi_i \rangle + \sum_{ik} \frac{4 p_i^2 p_k}{(p_i + p_k)^2} \beta_{ik,\nu} \beta_{ki,\mu}.
\end{aligned} \tag{6}$$

By antisymmetrizing the indices of the MSQGT, one obtains its imaginary part, namely,

$$Q_{[\nu\mu]} := \frac{1}{2}(Q_{\nu\mu} - Q_{\mu\nu}) = \frac{1}{2}(g_{\nu\mu} + i\sigma_{\nu\mu} - g_{\mu\nu} - i\sigma_{\mu\nu}) = \frac{1}{2} 2i\sigma_{\nu\mu} = i\sigma_{\nu\mu}, \tag{7}$$

where $[\cdot\cdot]$ denotes the antisymmetrization of the indices. $g$ and $\sigma$ represent the real part and imaginary part of $Q$, repectively. We have exploited the fact that $g_{\nu\mu}$ is symmetric and $\sigma_{\nu\mu}$ is anti-symmetric under the exchange of $\nu$ and $\mu$. Therefore

$$\sigma_{\nu\mu} = -iQ_{[\nu\mu]} = -i \left( \sum_i p_i \langle \partial_{[\nu} \xi_i | \partial_{\mu]} \xi_i \rangle + \sum_{ik} \frac{4 p_i^2 p_k}{(p_i + p_k)^2} \beta_{ik,[\nu} \beta_{ki,\mu]} \right). \tag{8}$$

In order to demonstrate that the imaginary part of the MSQGT is equivalent to the mean gauge curvature, we need to first compute the expression for $\langle \psi | D_\nu D_\mu | \psi \rangle$. Then antisymmetrizing the indices $\mu, \nu$ yields the corresponding expression for the mean gauge curvature $\langle \psi | T_{\nu\mu} | \psi \rangle$ using $T_{\nu\mu} = i[D_\nu, D_\mu]$. According to the definition of the covariant derivative, we have $\langle D_\nu D_\mu | \psi \rangle = \langle \psi | \partial_\nu | D_\mu \psi \rangle - \langle \psi | i\mathcal{A}_\nu | D_\mu \psi \rangle$. Next, we proceed to evaluate these two terms separately.

First, the connection, in the notation introduced above, can be expressed as

$$\begin{aligned} -i\mathcal{A}_\mu &= -I \otimes \sum_i \left( |\partial_\mu v_i\rangle\langle v_i| + \sum_k \frac{2\sqrt{p_i p_k}}{p_i + p_k} \langle \xi_k|\partial_\mu \xi_i\rangle |v_i\rangle\langle v_k| \right) \\ &= -I \otimes \sum_i |\partial_\mu v_i\rangle\langle v_i| - I \otimes \sum_{ik} \alpha_{ik}\beta_{ki,\mu} |v_i\rangle\langle v_k| \\ &= -I \otimes \sum_j |\partial_\mu v_j\rangle\langle v_j| - I \otimes \sum_{jl} \alpha_{jl}\beta_{lj,\mu} |v_j\rangle\langle v_l|, \end{aligned} \tag{9}$$

where $I$ is the identity matrix. Then

$$-i\mathcal{A}_\mu|\psi\rangle = -\sum_i \sqrt{p_i}|\xi_i\rangle|\partial_\mu v_i\rangle - \sum_{ij} \sqrt{p_i}\alpha_{ji}\beta_{ij,\mu}|\xi_i\rangle|v_j\rangle = -\sum_i \sqrt{p_i}|\xi_i\rangle|\partial_\mu v_i\rangle - \sum_{ik} \sqrt{p_i}\alpha_{ki}\beta_{ik,\mu}|\xi_i\rangle|v_k\rangle. \tag{10}$$

The covariant derivative is

$$\begin{aligned} D_\mu|\psi\rangle &= \partial_\mu|\psi\rangle - i\mathcal{A}_\mu|\psi\rangle \\ &= \sum_i \partial_\mu\sqrt{p_i}|\xi_i\rangle|v_i\rangle + \sum_i \sqrt{p_i}|\partial_\mu\xi_i\rangle|v_i\rangle + \sum_i \sqrt{p_i}|\xi_i\rangle|\partial_\mu v_i\rangle \\ &- \sum_i \sqrt{p_i}|\xi_i\rangle|\partial_\mu v_i\rangle - \sum_{ik} \sqrt{p_i}\alpha_{ki}\beta_{ik,\mu}|\xi_i\rangle|v_k\rangle \\ &= \sum_i \partial_\mu\sqrt{p_i}|\xi_i\rangle|v_i\rangle + \sum_i \sqrt{p_i}|\partial_\mu\xi_i\rangle|v_i\rangle - \sum_{ik} \sqrt{p_i}\alpha_{ki}\beta_{ik,\mu}|\xi_i\rangle|v_k\rangle \\ &= \sum_i \partial_\mu\sqrt{p_i}|\xi_i\rangle|v_i\rangle - \sum_{ik} \sqrt{p_k}\alpha_{ik}\beta_{ki,\mu}|\xi_k\rangle|v_i\rangle + \sum_i \sqrt{p_i}|\partial_\mu\xi_i\rangle|v_i\rangle. \end{aligned} \tag{11}$$

Then

$$\begin{aligned} \partial_\nu D_\mu|\psi\rangle &= \sum_i \partial_\mu\partial_\nu\sqrt{p_i}|\xi_i\rangle|v_i\rangle + \sum_i \partial_\mu\sqrt{p_i}|\partial_\nu\xi_i\rangle|v_i\rangle + \sum_i \partial_\mu\sqrt{p_i}|\xi_i\rangle|\partial_\nu v_i\rangle \\ &- \sum_{ik} \partial_\nu(\alpha_{ik}\sqrt{p_k})\beta_{ki,\mu}|\xi_k\rangle|v_i\rangle - \sum_{ik} \alpha_{ik}\sqrt{p_k}\partial_\nu\beta_{ki,\mu}|\xi_k\rangle|v_i\rangle \\ &- \sum_{ik} \alpha_{ik}\sqrt{p_k}\beta_{ki,\mu}|\partial_\nu\xi_k\rangle|v_i\rangle - \sum_{ik} \alpha_{ik}\sqrt{p_k}\beta_{ki,\mu}|\xi_k\rangle|\partial_\nu v_i\rangle \\ &+ \sum_i \partial_\nu\sqrt{p_i}|\partial_\mu\xi_i\rangle|v_i\rangle + \sum_i \sqrt{p_i}|\partial_\nu\partial_\mu\xi_i\rangle|v_i\rangle + \sum_i \sqrt{p_i}|\partial_\mu\xi_i\rangle|\partial_\nu v_i\rangle. \end{aligned} \tag{12}$$

Consequently

$$\begin{aligned} \langle\psi|\partial_\nu D_\mu|\psi\rangle &= \sum_i \sqrt{p_i}\partial_\mu\partial_\nu\sqrt{p_i} + \sum_i \sqrt{p_i}\partial_\mu\sqrt{p_i}\beta_{ii,\nu} + \sum_i \sqrt{p_i}\partial_\nu\sqrt{p_i}\beta_{ii,\mu} + \sum_i p_i\langle\xi_i|\partial_\nu\partial_\mu\xi_i\rangle \\ &+ \sum_i \sqrt{p_i}\partial_\mu\sqrt{p_i}\gamma_{ii,\nu} - \sum_{ik} \sqrt{p_k}\alpha_{ik}\sqrt{p_k}\beta_{ki,\mu}\gamma_{ki,\nu} + \sum_{ik} \sqrt{p_i p_k}\beta_{ki,\mu}\gamma_{ki,\nu} \\ &- \sum_i \sqrt{p_i}\partial_\nu\sqrt{p_i}\beta_{ii,\mu} - \sum_i p_i\partial_\nu\beta_{ii,\mu} - \sum_{ik} \sqrt{p_i}\alpha_{ik}\sqrt{p_k}\beta_{ki,\mu}\beta_{ik,\nu} \\ &= \sum_i \sqrt{p_i}\partial_\mu\partial_\nu\sqrt{p_i} + \sum_i (\sqrt{p_i}\partial_\mu\sqrt{p_i}\beta_{ii,\nu} + \sqrt{p_i}\partial_\nu\sqrt{p_i}\beta_{ii,\mu}) \\ &+ \sum_i \sqrt{p_i}\partial_\mu\sqrt{p_i}\gamma_{ii,\nu} - \sum_{ik} \sqrt{p_k}\alpha_{ik}\sqrt{p_k}\beta_{ki,\mu}\gamma_{ki,\nu} + \sum_{ik} \sqrt{p_i p_k}\beta_{ki,\mu}\gamma_{ki,\nu} \\ &- \sum_i \sqrt{p_i}\partial_\nu\sqrt{p_i}\beta_{ii,\mu} - \sum_i p_i\langle\partial_\nu\xi_i|\partial_\mu\xi_i\rangle - \sum_{ik} \sqrt{p_i}\alpha_{ik}\sqrt{p_k}\beta_{ki,\mu}\beta_{ik,\nu}. \end{aligned} \tag{13}$$

In the expansion of $\langle\psi|\partial_\nu D_\mu|\psi\rangle$, the terms in the first line are symmetric; after anti-symmetrization, they vanish and can be disregarded. Moreover, as we will show later, the terms in the second line are canceled by those in $\langle\psi| - i\mathcal{A}_\nu D_\mu|\psi\rangle$.

According to

$$-i\mathcal{A}_\nu = -I \otimes \sum_j |\partial_\nu v_j\rangle\langle v_j| - I \otimes \sum_{jl} \alpha_{jl}\beta_{lj,\nu}|v_j\rangle\langle v_l|, \tag{14}$$

we can obtain

$$\begin{aligned} -i\mathcal{A}_\nu D_\mu|\psi\rangle = &-\sum_i \partial_\mu\sqrt{p_i}|\xi_i\rangle|\partial_\nu v_i\rangle + \sum_{ik}\alpha_{ik}\sqrt{p_k}\beta_{ki,\mu}|\xi_k\rangle|\partial_\nu v_i\rangle - \sum_i \sqrt{p_i}|\partial_\mu\xi_i\rangle|\partial_\nu v_i\rangle \\ &-\sum_{ij}\alpha_{ji}\beta_{ij,\nu}\partial_\mu\sqrt{p_i}|\xi_i\rangle|v_j\rangle + \sum_{ijk}\alpha_{ji}\beta_{ik,\nu}\alpha_{ik}\sqrt{p_k}\beta_{ki,\mu}|\xi_k\rangle|v_j\rangle \\ &-\sum_{ij}\alpha_{ji}\beta_{ij,\nu}\sqrt{p_i}|\partial_\mu\xi_i\rangle|v_j\rangle. \end{aligned} \tag{15}$$

$$\begin{aligned} \langle\psi| - i\mathcal{A}_\nu D_\mu|\psi\rangle = &-\sum_i \sqrt{p_i}\partial_\mu\sqrt{p_i}\gamma_{ii,\nu} + \sum_{ik}\sqrt{p_k}\alpha_{ik}\sqrt{p_k}\beta_{ki,\mu}\gamma_{ki,\nu} - \sum_{ik}\sqrt{p_i p_k}\beta_{ki,\mu}\gamma_{ki,\nu} \\ &-\sum_i \sqrt{p_i}\beta_{ii,\nu}\partial_\mu\sqrt{p_i} + \sum_{ik}\sqrt{p_k}\alpha_{ki}\beta_{ik,\nu}\alpha_{ik}\sqrt{p_k}\beta_{ki,\mu} - \sum_{ik}\sqrt{p_k}\alpha_{ki}\beta_{ik,\nu}\sqrt{p_i}\beta_{ki,\mu}. \end{aligned} \tag{16}$$

The first line of Eq. (16) cancels with the second line of Eq. (13). Moreover, the first term in the second line of Eq. (16) and the first term in the third line of Eq. (13) combine into a symmetric term about $\mu$ and $\nu$, which vanishes upon anti-symmetrization. Therefore, by adding the two expressions and applying anti-symmetrization, we obtain

$$\begin{aligned} \langle\psi|D_{[\nu}D_{\mu]}|\psi\rangle &= \frac{1}{2}[\langle\psi|D_\nu D_\mu|\psi\rangle - \langle\psi|D_\mu D_\nu|\psi\rangle] \\ &= \frac{1}{2}\langle\psi|[D_\nu, D_\mu]|\psi\rangle \\ &= -\sum_i p_i\langle\partial_{[\nu}\xi_i|\partial_{\mu]}\xi_i\rangle + \sum_{ik}(-2\sqrt{p_i p_k}\alpha_{ik} + p_k\alpha_{ki}\alpha_{ik})\beta_{ik,[\nu}\beta_{ki,\mu]} \\ &= -\sum_i p_i\langle\partial_{[\nu}\xi_i|\partial_{\mu]}\xi_i\rangle + \sum_{ik}\frac{-4p_i p_k(p_i+p_k) + 4p_i p_k^2}{(p_i+p_k)^2}\beta_{ik,[\nu}\beta_{ki,\mu]} \\ &= -\sum_i p_i\langle\partial_{[\nu}\xi_i|\partial_{\mu]}\xi_i\rangle - \sum_{ik}\frac{4p_i^2 p_k}{(p_i+p_k)^2}\beta_{ik,[\nu}\beta_{ki,\mu]}. \end{aligned} \tag{17}$$

According to (8), we can obtain

$$\sigma_{\nu\mu} = i\langle\psi|D_{[\nu}D_{\mu]}|\psi\rangle = \frac{1}{2}\langle\psi|i[D_\nu, D_\mu]|\psi\rangle = \frac{1}{2}\langle\psi|T_{\mu\nu}|\psi\rangle, \tag{18}$$

where we have used the Eq. (23) in the main text.

* ben.wang@nju.edu.cn
† lijian.zhang@nju.edu.cn
